# Supplementary material for: A Reinforcement Learning Based Encoder-Decoder Framework for Learning Stock Trading Rules
Source: arXiv:2101.03867 source file (2021-01-08)
Supplement: Supplementary file 1 [file Appendix.tex]

\appendices

\section{Rules by the traditional rule-based agent}

\section{Rules by the SARSA($\lambda$) agent}

\section{Rules by the DQN agent}
